# Supplementary material for: From 'Here' to 'There': Exploring Proximity Semantics in Multimodal Data Exploration
Source: arXiv:2605.02261 source file (2026-05-04)
Supplement: Supplementary file 1 [file 8-appendix1.tex]

The user-settable penalties described here affect the segment similarity scores that lead to the final sketch-matching results, and are the primary mechanism for controlling how \harold~interprets a sketch.  

\begin{table}[h]
    \centering
    \begin{tabular}{|l|l|}
        \hline % Top horizontal line
        \textbf{Penalty} & \textbf{Purpose} \\

        \hline
        Length (Scale) Penalty & 
        \parbox[t]{10cm}{ % <-- \parbox is used here for wrapping and left justification
            Increasing this value penalizes differences in segment size, causing the system to find signals whose matched segments are the same size. Decreasing this penalty allows the system to include signals whose matched segments are differently sized.
        } \\
        
        \hline % Line separating headers from data
        Midpoint (Translation) Penalty & 
        \parbox[t]{10cm}{ % <-- \parbox is used here for wrapping and left justification
            Increasing this value penalizes differences in spatial position, causing the system to find signals in the same spatial area as the sketch. Decreasing this penalty allows the system to include more distal signals.
        } \\

        \hline
        Time Penalty & 
        \parbox[t]{10cm}{ % <-- \parbox is used here for wrapping and left justification
            Increasing this value penalizes differences in segment position along the time axis (which may or may not be visualized), causing the system to find signals occurring at the same time as the sketch. Decreasing this penalty value allows the system to include signals from other temporal regions of the data set.
        } \\
        
        \hline
        Velocity (Slope) Penalty & 
        \parbox[t]{10cm}{ % <-- \parbox is used here for wrapping and left justification
            Per-measure velocity is the change in a non-time measure divided by the change in time. For univariate time series data such as baby name popularity, the \textit{x} axis \textit{is} time. As a result, the signal velocity (d\textit{y}/d\textit{x}) \textit{is the slope of the line}.  Thus, for univariate signals, the velocity penalty scalar affects the degree to which segment slope is matched. For non-univariate signals like storm tracks, velocities are still calculated but may not be visually shown. Increasing this penalty value penalizes differences in segment velocity, causing the system to find signals with similar signal velocities. Decreasing this penalty value allows the system to include signals with less-similar signal velocities.
        } \\

        \hline
        Skipped Segment Penalty & 
        \parbox[t]{10cm}{ % <-- \parbox is used here for wrapping and left justification
            Often, two signals have a very similar shape but differ in the exact segment count (e.g., Figure \ref{fig:geom_sketch_arch}C S1-S3 and \ref{fig:geom_sketch_arch}D B1-B2). Segment skipping allows the system to make the best match (e.g., S1:B1, S3:B2) and skip the intervening segment (S2). Without segment skipping, segments S2 and B2 would be forced to match, which would generate a large error value and is intuitively incorrect. The Skipped Segment Penalty determines the cost of segment skipping; increasing it discourages segment skipping, encouraging a precise segment:segment signal match, while decreasing it encourages segment skipping, allowing a more flexible signal matching.
        } \\

        \hline
        Segment Count Penalty & 
        \parbox[t]{10cm}{ % <-- \parbox is used here for wrapping and left justification
            Increasing this value penalizes differences in per-signal segment count, causing the system to find signals with the same number of segments. Decreasing this penalty allows the system to include signals with increasingly different segment counts. Adjusting this penalty can help the user control overall shape matching.
        } \\

        \hline
        Stretch Penalty & 
        \parbox[t]{10cm}{ % <-- \parbox is used here for wrapping and left justification
            Adjusting this penalty will determine if the sketched line is used to find a sub-shape of a signal or the entire shape of a signal. Consider the sketched line in Figure \ref{fig:geom_sketch_arch}A.1. If the stretch penalty value is high, the lowest-penalty signals will be those whose entire shape matches the sketch, i.e., the signals whose first segment matches the sketch's first segment and whose last segment matches the sketch's last segment. If, however, this penalty value is low, then the system will allow signals that simply \textit{include} the sketched shape i.e. signals that may include this path but which start before the sketch's start and continue after the sketch's end.
            \\
        } \\
        
        \hline % Bottom horizontal line
    \end{tabular}
    \caption{User-settable Penalties}
    \label{tab:user-dofs}
\end{table}
