# Supplementary material for: From 'Here' to 'There': Exploring Proximity Semantics in Multimodal Data Exploration
Source: arXiv:2605.02261 source file (2026-05-04)
Supplement: Supplementary file 2 [file supp.tex]

% ---------------------------------------------------------------------------
% Author guideline and sample document for EG publication using LaTeX2e input
% D.Fellner, v1.21, Jan 08, 2024

\documentclass{egpubl}
\usepackage{eurovis2026}

\EuroVisShort  % for EuroVis additional material
% \MedicalPrize  % uncomment for Medical Prize (Dirk Bartz) contribution, since 2021 part of EuroVis
% \EuroVisEducation              % uncomment for Education contribution

% Licences: for CGF Journal (EG conf. full papers and STARs, EuroVis conf. full papers and STARs, SR, SGP, PG)
% please choose the correct license
%\CGFStandardLicense
%\CGFccby
%\CGFccbync
%\CGFccbyncnd

% !! *please* don't change anything above
% !! unless you REALLY know what you are doing
% ------------------------------------------------------------------------
\usepackage[T1]{fontenc}
\usepackage{dfadobe}
\usepackage{amsmath} 
\usepackage[hyphens,spaces,obeyspaces]{url}

\usepackage{cite}  % comment out for biblatex with backend=biber
% ---------------------------
%\biberVersion
\BibtexOrBiblatex
%\usepackage[backend=biber,bibstyle=EG,citestyle=alphabetic,backref=true]{biblatex}
%\addbibresource{egbibsample.bib}
% ---------------------------
\electronicVersion
\PrintedOrElectronic
% for including postscript figures
% mind: package option 'draft' will replace PS figure by a filename within a frame
\ifpdf \usepackage[pdftex]{graphicx} \pdfcompresslevel=9
\else \usepackage[dvips]{graphicx} \fi

\usepackage{egweblnk}

\input{supp.inc}
