# Supplementary material for: From 'Here' to 'There': Exploring Proximity Semantics in Multimodal Data Exploration
Source: arXiv:2605.02261 source file (2026-05-04)
Supplement: Supplementary file 3 [file system.tex]

\section{Implementation Overview}
The research probe is implemented as a web application. The frontend is built using \href{https://react.dev}{React.js} and \href{https://www.typescriptlang.org}{TypeScript}, and includes an HTML5 canvas for free-form sketch input, along with \href{https://d3js.org}{D3} and \href{https://www.mapbox.com}{Mapbox} for rendering time-series and geospatial visualizations. The backend uses \href{https://www.postgresql.org}{PostgreSQL 16.6} for structured data storage and processing, with \href{https://nodejs.org}{Node.js} and \href{https://www.python.org}{Python 3.12} coordinating API services and multimodal processing. Language and visual annotation interpretation are supported by the \href{https://github.com/openai/openai-node}{OpenAI JavaScript API} and \href{https://www.anthropic.com/claude}{Anthropic Claude 3.7 Sonnet}.



\section{Geometric Analysis and Trend Search}\label{geomsearch}
Building on the implementation context described above, this section summarizes the geometric processing steps used by the research probe to support sketch-based trend search (Figure 2 in the paper). The pipeline converts both database-resident signals and user-drawn sketches into comparable geometric representations, enabling similarity-based retrieval and exploration. The following steps are performed on the data in the database.

\textbf{Initial data.} The probe supports time-series datasets that include a continuous datetime attribute, one or more categorical dimensions, and at least one continuous measure. These signals serve as the input for both database indexing and sketch-based querying.

\textbf{Normalization.} All continuous data measures are normalized to the range of $[0,1]$ prior to analysis. The probe supports two normalization modes: \textit{local normalization} in which each signal is scaled based on its own minimum and maximum values, and \textit{global normalization} in which all signals are scaled using an externally-determined min–max range. This allows users to emphasize either relative shape or absolute magnitude during search.

\textbf{Signal segmentation.} Signals are then simplified using Douglas–Peucker linear segmentation, producing a piecewise-linear approximation within user-defined error tolerances. This step reduces signal complexity while preserving salient structural features needed for comparison. 

\textbf{Per-segment signal property analysis.} For each resulting segment, the probe computes a small set of geometric and temporal descriptors, including segment length, spatial midpoint, temporal midpoint, and velocity. These descriptors form a compact representation that supports localized comparison between signals.

\textbf{Signal alignment.} Similarity between two simplified signals is computed by aligning their segments and accumulating a difference score based on corresponding segment descriptors. The alignment follows a standard dynamic programming formulation over a segment-to-segment distance matrix, producing a least-error correspondence between segments. A score of zero indicates exact structural equivalence. Several user-adjustable penalty terms (shown in Section \S\ref{sec:penalties}) influence this calculation, allowing users to control sensitivity to differences in scale, position, timing, and slope.


\textbf{Signal clustering.} To help users explore the dominant shape patterns present in their data, the probe also performs signal clustering. Pairwise distances between signals are computed using the same geometric similarity metric, and agglomerative clustering is applied to identify common shape patterns in the data. For each cluster, the medoid signal is selected as a visual representative of the dominant trend shape.

Trend search applies this same processing pipeline to a user-drawn sketch. After sketch input, the drawn shape is simplified, analyzed, and compared against the indexed database signals. Signals with the lowest geometric difference scores are returned as the best matches and presented to the user.

\section{Free-form and Natural Language Annotation}
In addition to geometric sketch matching, the research probe supports free-form and natural language annotations that allow users to express semantic and analytical constraints. Multimodal user inputs, including sketches, text, and visual annotations, are consolidated into a single composite image and passed to a backend visual language model (VLM) along with contextual metadata. The VLM parses the image and produces a structured representation of the user's constraints, which is translated into executable SQL. The resulting query output is then logically intersected with the results of the geometric sketch search to form the final returned dataset. To support reliable interpretation, the following metadata is provided to the VLM (see supplementary example files for the full prompts):

%Here is the metadata that is sent to the VLM.

\textbf{High-level planning instructions.} The VLM is provided with explicit guidance describing its role as a visual parsing and analytic reasoning agent, along with a high-level sequence of subtasks such as image analysis, directive interpretation, and SQL query composition.

\textbf{Schema-aware semantic grounding.} Schema-level information, including field names and expected value types, is provided to ground annotations in the underlying data representation and reduce ambiguity during interpretation.

\textbf{Visual orientation context.} Each composite image is augmented with visual orientation cues, such as latitude/longitude geographic references or axis markers.

\textbf{Glyph interpretation directives.} The VLM is informed of the intended semantics of commonly used visual glyphs such as inclusion circles, exclusion cross-outs, boundary lines, and arrows. Instructions are also provided for handling ambiguous or novel inputs. 

\textbf{SQL generation guidance.} The prompt includes constraints and formatting guidance to ensure that generated SQL queries are syntactically valid and aligned with the database schema. 


\clearpage
\section{User-settable Penalties}
\label{sec:penalties}

The user-settable penalties described here expose implementation-level parameters that allow users to adjust the behavior of geometric matching in the probe during exploration.

\begin{table}[h]
    \centering
    \begin{tabular}{|l|l|}
        \hline % Top horizontal line
        \textbf{Penalty} & \textbf{Purpose} \\

        \hline
        Length (Scale) Penalty & 
        \parbox[t]{10cm}{ % <-- \parbox is used here for wrapping and left justification
            Increasing this value penalizes differences in segment size, causing the system to find signals whose matched segments are the same size. Decreasing this penalty allows the system to include signals whose matched segments are differently sized.
        } \\
        
        \hline % Line separating headers from data
        Midpoint (Translation) Penalty & 
        \parbox[t]{10cm}{ % <-- \parbox is used here for wrapping and left justification
            Increasing this value penalizes differences in spatial position, causing the system to find signals in the same spatial area as the sketch. Decreasing this penalty allows the system to include more distal signals.
        } \\
        

        
        \hline
        Time Penalty & 
        \parbox[t]{10cm}{ % <-- \parbox is used here for wrapping and left justification
            Increasing this value penalizes differences in segment position along the time axis (which may or may not be visualized), causing the system to find signals occurring at the same time as the sketch. Decreasing this penalty value allows the system to include signals from other temporal regions of the data set.
        } \\
        
        \hline
        Velocity (Slope) Penalty & 
        \parbox[t]{10cm}{ % <-- \parbox is used here for wrapping and left justification
            Per-measure velocity is the change in a non-time measure divided by the change in time. For univariate time series data such as baby name popularity, the \textit{x} axis \textit{is} time. As a result, the signal velocity (d\textit{y}/d\textit{x}) \textit{is the slope of the line}.  Thus, for univariate signals, the velocity penalty scalar affects the degree to which segment slope is matched. For non-univariate signals like storm tracks, velocities are still calculated but may not be visually represented. Increasing this penalty value penalizes differences in segment velocity, causing the system to find signals with similar signal velocities. Decreasing this penalty value allows the system to include signals with less-similar signal velocities.
        } \\

        \hline
        Skipped Segment Penalty & 
        \parbox[t]{10cm}{ % <-- \parbox is used here for wrapping and left justification
            Often, two signals have a very similar shape but differ in the exact segment count (e.g., in the paper, Figure 2C S1-S3 and 2D B1-B2). Segment skipping allows the system to make the best match (e.g., S1:B1, S3:B2) and skip the intervening segment (S2). Without segment skipping, segments S2 and B2 would be forced to match, which would generate a large error value and is intuitively incorrect. The Skipped Segment Penalty determines the cost of segment skipping; increasing it discourages segment skipping, encouraging a precise segment:segment signal match, while decreasing it encourages segment skipping, allowing a more flexible signal matching.
        } \\

        \hline
        Segment Count Penalty & 
        \parbox[t]{10cm}{ % <-- \parbox is used here for wrapping and left justification
            Increasing this value penalizes differences in per-signal segment count, causing the system to find signals with the same number of segments. Decreasing this penalty allows the system to include signals with increasingly different segment counts. Adjusting this penalty can help the user control overall shape matching.
        } \\

        \hline
        Stretch Penalty & 
        \parbox[t]{10cm}{ % <-- \parbox is used here for wrapping and left justification
            Adjusting this penalty will determine if the sketched line is used to find a sub-shape of a signal or the entire shape of a signal. Consider the sketched line in the paper, Figure 2A.1. If the stretch penalty value is high, the lowest-penalty signals will be those whose entire shape matches the sketch, i.e., the signals whose first segment matches the sketch's first segment and whose last segment matches the sketch's last segment. If, however, this penalty value is low, then the system will allow signals that simply \textit{include} the sketched shape i.e., signals that may include this path but which start before the sketch's start and continue after the sketch's end.
            \\
        } \\
        
        \hline % Bottom horizontal line
    \end{tabular}
    \caption{User-settable Penalties}
    \label{tab:user-dofs}
\end{table}
